# Supplementary material for: RAMP: A Flat Nanosecond Optical Network and MPI Operations for Distributed Deep Learning Systems
Source: arXiv:2211.15226 source file (2023-02-24)
Supplement: Supplementary file 1 [file appendix.tex]

\clearpage
\newpage

\section{Appendix}

\input{Tables/RAMP-Basic}
\subsection{Architecture parameters}
\label{sec:architecture_parameters}
Table \ref{tab:Parameters_all} gives a detailed representation of the design parameters for the proposed topologies, continuing the description performed in \S \ref{RAMP} and Table I. 

It shows how the system and network properties scale with each of the parameters. The combined information provided in Table \ref{tab:Parameters_all} and Table \ref{tab:subnet} give a complete representation of all the possible configurations of the system. In addition, the formulae provided are at the core of the power budget calculation which were used to produce Fig. \ref{fig:power}. For Fig. \ref{fig:power} the SOA gain and the AWGR insertion loss have been considered to be 21~dB and 5~dB respectively.

% \subsection{Subnet Comparison}
% Table \ref{tab:subnet} shows the characteristics of each subnet in terms of components and optical properties.

% \input{Tables/transceiver_selection}
% \input{Tables/SubnetComparison}
\subsection{Contention}
\label{contention}
In the proposed RAMP architectures, each sub-net hosts the communication between specific ($i^{th}$) transmitter and receiver between a source and destination communication group. Each communication group contains $J$ racks with $\Lambda$ devices per rack. Due to the fact that there are only $\Lambda$ available wavelength channels within the sub-net, there would be more requests of source-destination node pairs than wavelengths per sub-network, which could potentially contend.

As each transmitter can talk to every receiver within the sub-net, and there are $x$ possible sub-nets which connect any source node to any destination node, the communication is rearrangeably non-blocking. This is the case because the maximum number of racks ($J$) is always lesser or equal to the number of transceivers  ($x$) between communication groups.

While all architectures are at least re-arrangeably non-blocking, the actual contention per sub-network varies depending upon the optical technology employed.

\subsubsection{B\&S}
In the broadcast and select architecture, the total number of communications that can be handled by an individual sub-network at any given time is $\Lambda$, irrespective of the transceiver/receiver type. This means that only $1/J$ (worst case $1/x$) of the available capacity can be used by any sub-network, making the effective contention probability $1/J$.

\subsubsection{R\&B}
In the route and broadcast sub-net, the contention is possible only in the coupler (broadcast) stage. Within each sub-net, the wavelength channels available in the system is always larger than the coupler (or contending path) size  ($\Lambda >  J$), allowing full capacity communication within a sub-net. However, when information from the same node number pairs across racks occurs, the same wavelength will have to be used within the same coupler leading to contention, leading to a maximum of $J$ contending communications. Although the contention of this sub-net is comparatively less to the B\&S sub-net, the numerical analysis of contention probability is out of the scope of this paper.

\input{Tables/SubnetComparison}
% In the RAMP architecture, the destination selection is performed in two  stages. In the first stage, the wavelength selects to which device in a rack they set the communication. In this stage there is no wavelength contention. At the second stage the signals of all the $\lambda^{th}$ ports of the $J$ AWGRs are coupled together, such that the signal from all the $\lambda^{th}$ ports is propagated to the $\lambda^{th}$ device of all the $J$ racks. In this stage there might be contention as same wavelength may be used for transmission in the same star coupler. This occurs when the input and the output port of multiple AWGRs is the same, limiting the contention to $J$ possible source destination pairs. 

% The contention will happen when there will be two or more source destination pairs such as any device $\lambda_{src}$ of any rack $j$ wants to communicate to device $\lambda_{dst}$ of rack $k$. This reduces the maximum contention to a $J \times J$ (up to $x \times x$) communication pairs. If the number of wavelengths and number of devices per rack $\Lambda \geq J$ it is possible to achieve full capacity communication between individual subnet.

% The characteristics of this architecture, contention is considered only between inter rack level, where there are up to $J$ source-destination pairs contending. The actual numerical evaluation of the blocking probability of this architecture 

\subsubsection{R\&S}
The route and switch subnet builds on the principle of R\&B, but replaces the couplers with SOA gated splitters and combiners. This feature increases the space division multiplexing, allowing the active selection of the destination rack. In this manner, inter rack contention is avoided, making the architecture contention free.

% \subsection{Job placement}
% To maximise the network utilisation and avoid contention between communicating nodes smart placement may be needed depending on the architecture and job.

\subsection{Power Consumption}
\label{app:power}
We perform a power analysis of the proposed system in comparison of EPS equivalent systems. We compare with architecture for HPC and DCN where we match the scale of the network in terms of number of nodes (65,536) and all-to-all node bandwidth (12.8~Tbps per node). We consider the Nvidia DGX-A100 SuperPod \cite{superpod} based architecture for HPC systems and a Fat-Tree network for DCN systems.

All the assumptions made to estimate the power consumption per each component and number of active components are shown in Table \ref{power_breakdown}. 

The values of Table \ref{power_breakdown} are used for the power analysis shown in Fig. \ref{fig:power_comp}. The power for all of RAMP's configurations is compared to bandwidth-per-node and scale matched electronic packet switched network counterparts. In terms of energy per bit, the propose system consumes from 7.7 (B\$S with fixed TX) to 9.5 (for R\&B) pJ/bit/path. In contrast, the HPC and DCN counterparts consume 382 and 363 pJ/bit/path respectively, which corresponds to a 38$\times$ minimum increase in energy per bit in respect to the proposed system. Similarly, in terms of overall power consumption, the RAMP system consumes from 6.4 to 8 MW whereas the EPS consumes $334$ and $339$ MW for HPC and DCN respectively. RAMP offers a 42-53$\times$ improvement in terms of overall energy consumption in respect of equivalent EPS systems.
% The switching devices and transceivers assumed for comparative EPS networks: (1) Nvidia DGX-A100 Superpod based network cluster and (2) a Fat-Tree DCN, both with equivalent node capacity (12.8~Tbps per node) and node numbers (65,536) are also included in the table. 

The QM8790 switch power consumption assumed in the NVidia SuperPod architecture is from \cite{mellanox_technologies_qm8790_2021}. The transceivers used are the 200 Gb/s MMF InfiniBand compatible transceiver and the corresponding power is taken from \cite{200g_tx}. For the fat-tree DCN, the switch assumed for all tiers is the Arista 7170 \cite{arista}. For small distances (1-tier), a QSFP28 100G transceiver is assumed \cite{short_tx} and for longer distances (higher tiers), the Arista 100G QSFP-SR4 is assumed \cite{long_tx}.

\input{Tables/table_power}

\begin{figure}[tp]
    \centering
    \includegraphics[width=\linewidth]{figures/Energy_comp.pdf}
    \caption{Energy comparison with equivalent EPS network.}
    \label{fig:power_comp}
\end{figure}

For the RAMP systems, the power consumption values are estimated for the fixed laser from \cite{non-tunable}, tunable laser from \cite{Dsdbr}, the modulator from \cite{mod1, mod2}, the receiver from \cite{pd}, the SOA and gated tunable filters from \cite{soa}.

\subsection{Scalability}
\label{app:scalability}
\begin{figure}[tp]
    \centering
    \includegraphics[width=\linewidth]{figures/Nodes_and_b_per_node_capacity.pdf}
    \caption{Scalability of architecture for node capacity keeping same amount of SOA.}
    \label{fig:nodes_vs_capacity}
\end{figure}
As shown in Table I, every node is equipped with $bx$ transceivers, where a group of $b$ transceivers are grouped together to communicate with the racks in 1 of $x$ communication groups. Unless otherwise mentioned in the paper, we have carried out our simulations and network analysis for $b=1$ and 65,536~nodes, which corresponds to each node having a capacity of 12.8~Tbps (=2.9375 TBps).
However, if an engineer prefers to deploy a custom RAMP-based network architecture with scalability emphasis on communication bandwidth density per node ($>$12.8~Tbps) than node count ($<$65,536 nodes), $b$ transceivers can be grouped to connect $b$ parallel sub-nets to the same communication group for the same number of optical gates. The values for the number of optical gates in each of the RAMP sub-nets can be seen in Table \ref{tab:subnet}. 

Fig. \ref{fig:nodes_vs_capacity} shows how the per-node capacity can be scaled with the same complexity (number of optical gates) with a compromise on the node-count. It can be noted that the R\&S system can achieve up to 120~TB/s (960~Tbps) node capacity supporting 6,400 nodes for the same number of optical gates as the 65,536 nodes at 12.8~Tbps mentioned in this paper. 
\begin{figure}[bp]
    \centering
    \includegraphics[width=\linewidth]{figures/Reduction comp.pdf}
    \caption{Computational time taken to sum 1GB of information scattered onto $\#GPUs$ workers, using algorithm having a single source and RAMP (multiple sources).}
    \label{fig:Compute-reduction}
\end{figure}
\begin{figure*}[hbp]
    \centering
    \includegraphics[width=\linewidth]{figures/allreduce_real_True.pdf}
    \caption{All-reduce completion time between system based on Nvidia DGX-A100 SuperPod and the RAMP architecture, varying number of nodes and message size.}
    \label{fig:allred_comp_real}
\end{figure*}

State-of-the art accelerators such as the Tesla DOJO tile~\cite{tesla}, which have a high I/O node capacity of up to 36 TB/s (288 Tbps), are interconnected in systems using 2D-Torus or meshes architectures due to large bandwidth constraints.  However, in such interconnections, the connectivity is limited and the effective bandwidth for communication between connected nodes is only a fraction of the overall capacity (a fourth of the overall capacity for 2D-torus). As seen in Fig. \ref{fig:nodes_vs_capacity} RAMP could allow a full-bisection, all-to-all connectivity between 12,544 DOJO tile accelerators, further proving the scalability of the system for high performance applications.

Moreover, the power consumption per path can be further reduced by employing a single laser source with a booster amplifier (SOA) and splitting it across to $b$ modulators. Although we acknowledge this benefit, our detailed power analysis (\S \ref{app:power}) in this section showcases a worst-case value while assuming $b=1$.

In Fig.\ref{fig:sota}, we compare the proposed system with state-of-the-art electronic packet switched systems (\cite{DELL, IBM, nvidia_dgx1, nvidia_dgx2, habana_labs_ltd__gaudi_2019, Philly, TaihuLight, TPU_pod}) and a proposed optical system (\cite{terarack}). The figure shows that we are able to achieve an increase of a factor from $40-400 \times$ in respect of custom platforms, while achieving a $20-16000 \times$ increase in bandwidth over HPC clusters.

\subsection{Computational Analysis}
\label{app:compute}
For the single source based collective operations, such as the ring or recursive halving or doubling ones, the reduction operation is performed sequentially between the local information and the incoming information, making the reduction operation a 2-to-1 operation which is largely memory limited. In contrast, in RAMP each device receives pieces of information from up to $x-1$ independent sources in parallel such that the reduction operation in each device is an x-to-1 operation. 

% The use of parallel reduction increases the arithmetic intensity of the operation therefore decreasing the total computation time. 

The improvement is shown in Fig \ref{fig:Compute-reduction} in which the time taken to sum 1~GB information spread across $n$ sources is plotted for sequential algorithms and parallel RAMP network. This operation leads to significant improvements in reduction time by a factor of up-to 2.8 times. 

Note that for all our calculations, we assume half-precision operations (16~bit) as it is widely used in DDL.

\subsection{Reliability comparison to OCS counterparts}
Compared to other ns-level circuit reconfiguration optical architectures such as PULSE \cite{Benjamin:20} and Sirius \cite{ballani2020sirius}, the RAMP architecture provides better network reliability. Owing to limited spatial path availability, both PULSE and Sirius network architectures suffer from single point failure in terms of transceiver and subnet. In fact, these architectures employ a single transceiver to connect one device to a specific rack (with $N$ devices) and a single subnet to interconnect any pair of racks. This means that if a transceiver in a node fails $N$ possible communications are not anymore available, and in the case of a subnet failure $N^2$ source-destination pairs of requests have lost access. In contrast, in RAMP there $b x$ possible paths interconnect any node pair, and $b x$ subnets interconnect any pair of communication groups. Because of this spatial parallelism, connectivity is still possible in case of failure, but with a lower data-rate ($bx -1$ active transceivers). In case of failure, the transceiver map formulation can be modified in a cyclic manner to optimise the collective completion time such that the faulty resource is not used within the MPI operations.

\subsection{Additional Results}
In Fig. \ref{fig:allred_comp_real}, the comparison between the proposed system and a system based on Nvidia DGX-A100 SuperPod \cite{superpod} architecture is performed.  It can be noted that the combination of the  proposed RAMP system and the RAMP-x MPI algorithm lead to a minimum speed-up over the EPS counterparts of 10$\times$ in completion time for All-Reduce operations. This is mainly attributed to the high data-rate between inter-rack nodes and the larger node capacity available in RAMP, proving the significance of having high bandwidth all-to-all communication. 

The increase in bandwidth has a larger effect on MPI operations that are data-transfer limited, where the overall message size does not vary between sub operations (consecutive hierarchies in hierarchical 2D-Torus, hierarchical ring algorithms and algorithmic steps in RAMP). An example is the all-to-all operation, where the RAMP algorithm and topology lead to a speed-up of a factor above 171$\times$, as shown in Fig.\ref{fig:collective_comp}.

\subsection{Circuit reconfiguration time}
\label{app:circ-rec}

The circuit reconfiguration delay is a fundamental factor to calculate the performance of the network. It determines the minimum message size that can be transmitted between pairs of node. This is especially important when dealing with small messages and/or large scale MPI collectives. When large number of devices are included in an MPI operation for certain collective operations (reduce-scatter, scatter, reduce), the message size transmitted per communication step by each device decreases with the number of devices involved. For example, at maximum scale (65,536 nodes), performing a reduce-scatter operation where each device needs to share 10~GB of data, will have to transmit a message of 152~kB in at least one communication steps. Considering an aggregate bandwidth of a node to be 12.8~Tbps, such a communication would require 95.4~ns. To achieve effective transmission, the circuit reconfiguration time should be $<5\%$ of the overall transmission time, which in this case, corresponds to 4.75~ns. As we can perform wavelength tunability and SOA gating in sub-ns regime, this communication is feasible. In RAMP, we assume minimum communication epoch (time-slot size) to be 20~ns, such that the minimum message size can vary from 950~B to 30.4~kB depending on the number of transceivers active per communication (from 1 to 32). The effective bandwidth required can be predetermined for each communication step, allowing only a subset of possible transceivers to be utilised, leading to lower power consumption and smaller network contention possibly increasing the number of active job in the system.

The all-to-all, full bandwidth, fast reconfiguration properties of RAMP architecture provides high performance tolerance to communication degree \cite{khani_mehrdad_2021}. The sub-ns reconfiguration is an essential property that enables RAMP to achieve high goodput with minimal reconfiguration overhead. As the optical circuit switches in RAMP can support a range of circuits (ns-hours), the use of algorithms such as the one described in \ref{coll_ops}, where the communication circuit varies between each algorithmic step is possible. These algorithms, with respect to the ones with fixed communication pattern (used for high circuit reconfiguration latency) such as ring based algorithms have significantly lower head-to-head (H2H) latency and lead to faster collective completion time as demonstrated in \S \ref{result}.

\input{Tables/teable_reconfig_latency}

In Table \ref{tab:rec_lat}, we show the impact of circuit reconfiguration time on a scatter collective completion time using different message sizes. Each row is normalised by the completion time when the reconfiguration delay is 0. It needs to be noticed that this correspond to a scatter operation job where the amount of algorithmic steps and therefore, circuit reconfigurations is 4. Table. \ref{tab:rec_lat} shows that as the circuit reconfiguration time increases, the collective completion time also increases. It can be seen that when the reconfiguration time is less than equal than the I/O latency (200 ns), the completion time stays constant. This is due to the fact that the circuit reconfiguration is performed at the same time as the information is processed inside the node. Therefore, to avoid additional overhead the circuit reconfiguration time should be smaller than the I/O latency. 
Whenever the reconfiguration delay is larger than the I/O latency, there is significant increase in the collective completion time. This is justified because the longer portion of the operation time is taken by the circuit reconfiguration. As the message size increases, the relative increase in completion time reduces as the larger portion of the completion time is taken by the data transfer. The value of 25$\mu$s and 10ms have been chosen as they correspond to the circuit reconfiguration time of \cite{khani_mehrdad_2021} considering a small scale Micro-Ring Resonator (MRR) based ring topology and large scale MEMS OCS topology respectively. For 25$\mu$s reconfiguration. the delay is significant for messages of sizes smaller than 10~GB (15\%-1690\% increase over the baseline) making a system with such reconfiguration time effective only for large messages. The 10~ms reconfiguration lead to 7.2-6412$\times$ increase in completion time, making it unfeasible for dynamic algorithms. 

Fast circuit reconfiguration is also required for handling dynamic traffic, where information from a node can be sent to multiple nodes sequentially without any collective operations. Future work will include the development of a scheduler for the proposed architectures to handle such traffic.
